# Supplementary material for: LayoutDiffusion: Improving Graphic Layout Generation by Discrete Diffusion Probabilistic Models
Source: arXiv:2303.11589 source file (2023-08-15)
Supplement: Supplementary file 1 [file type_rico.pdf]

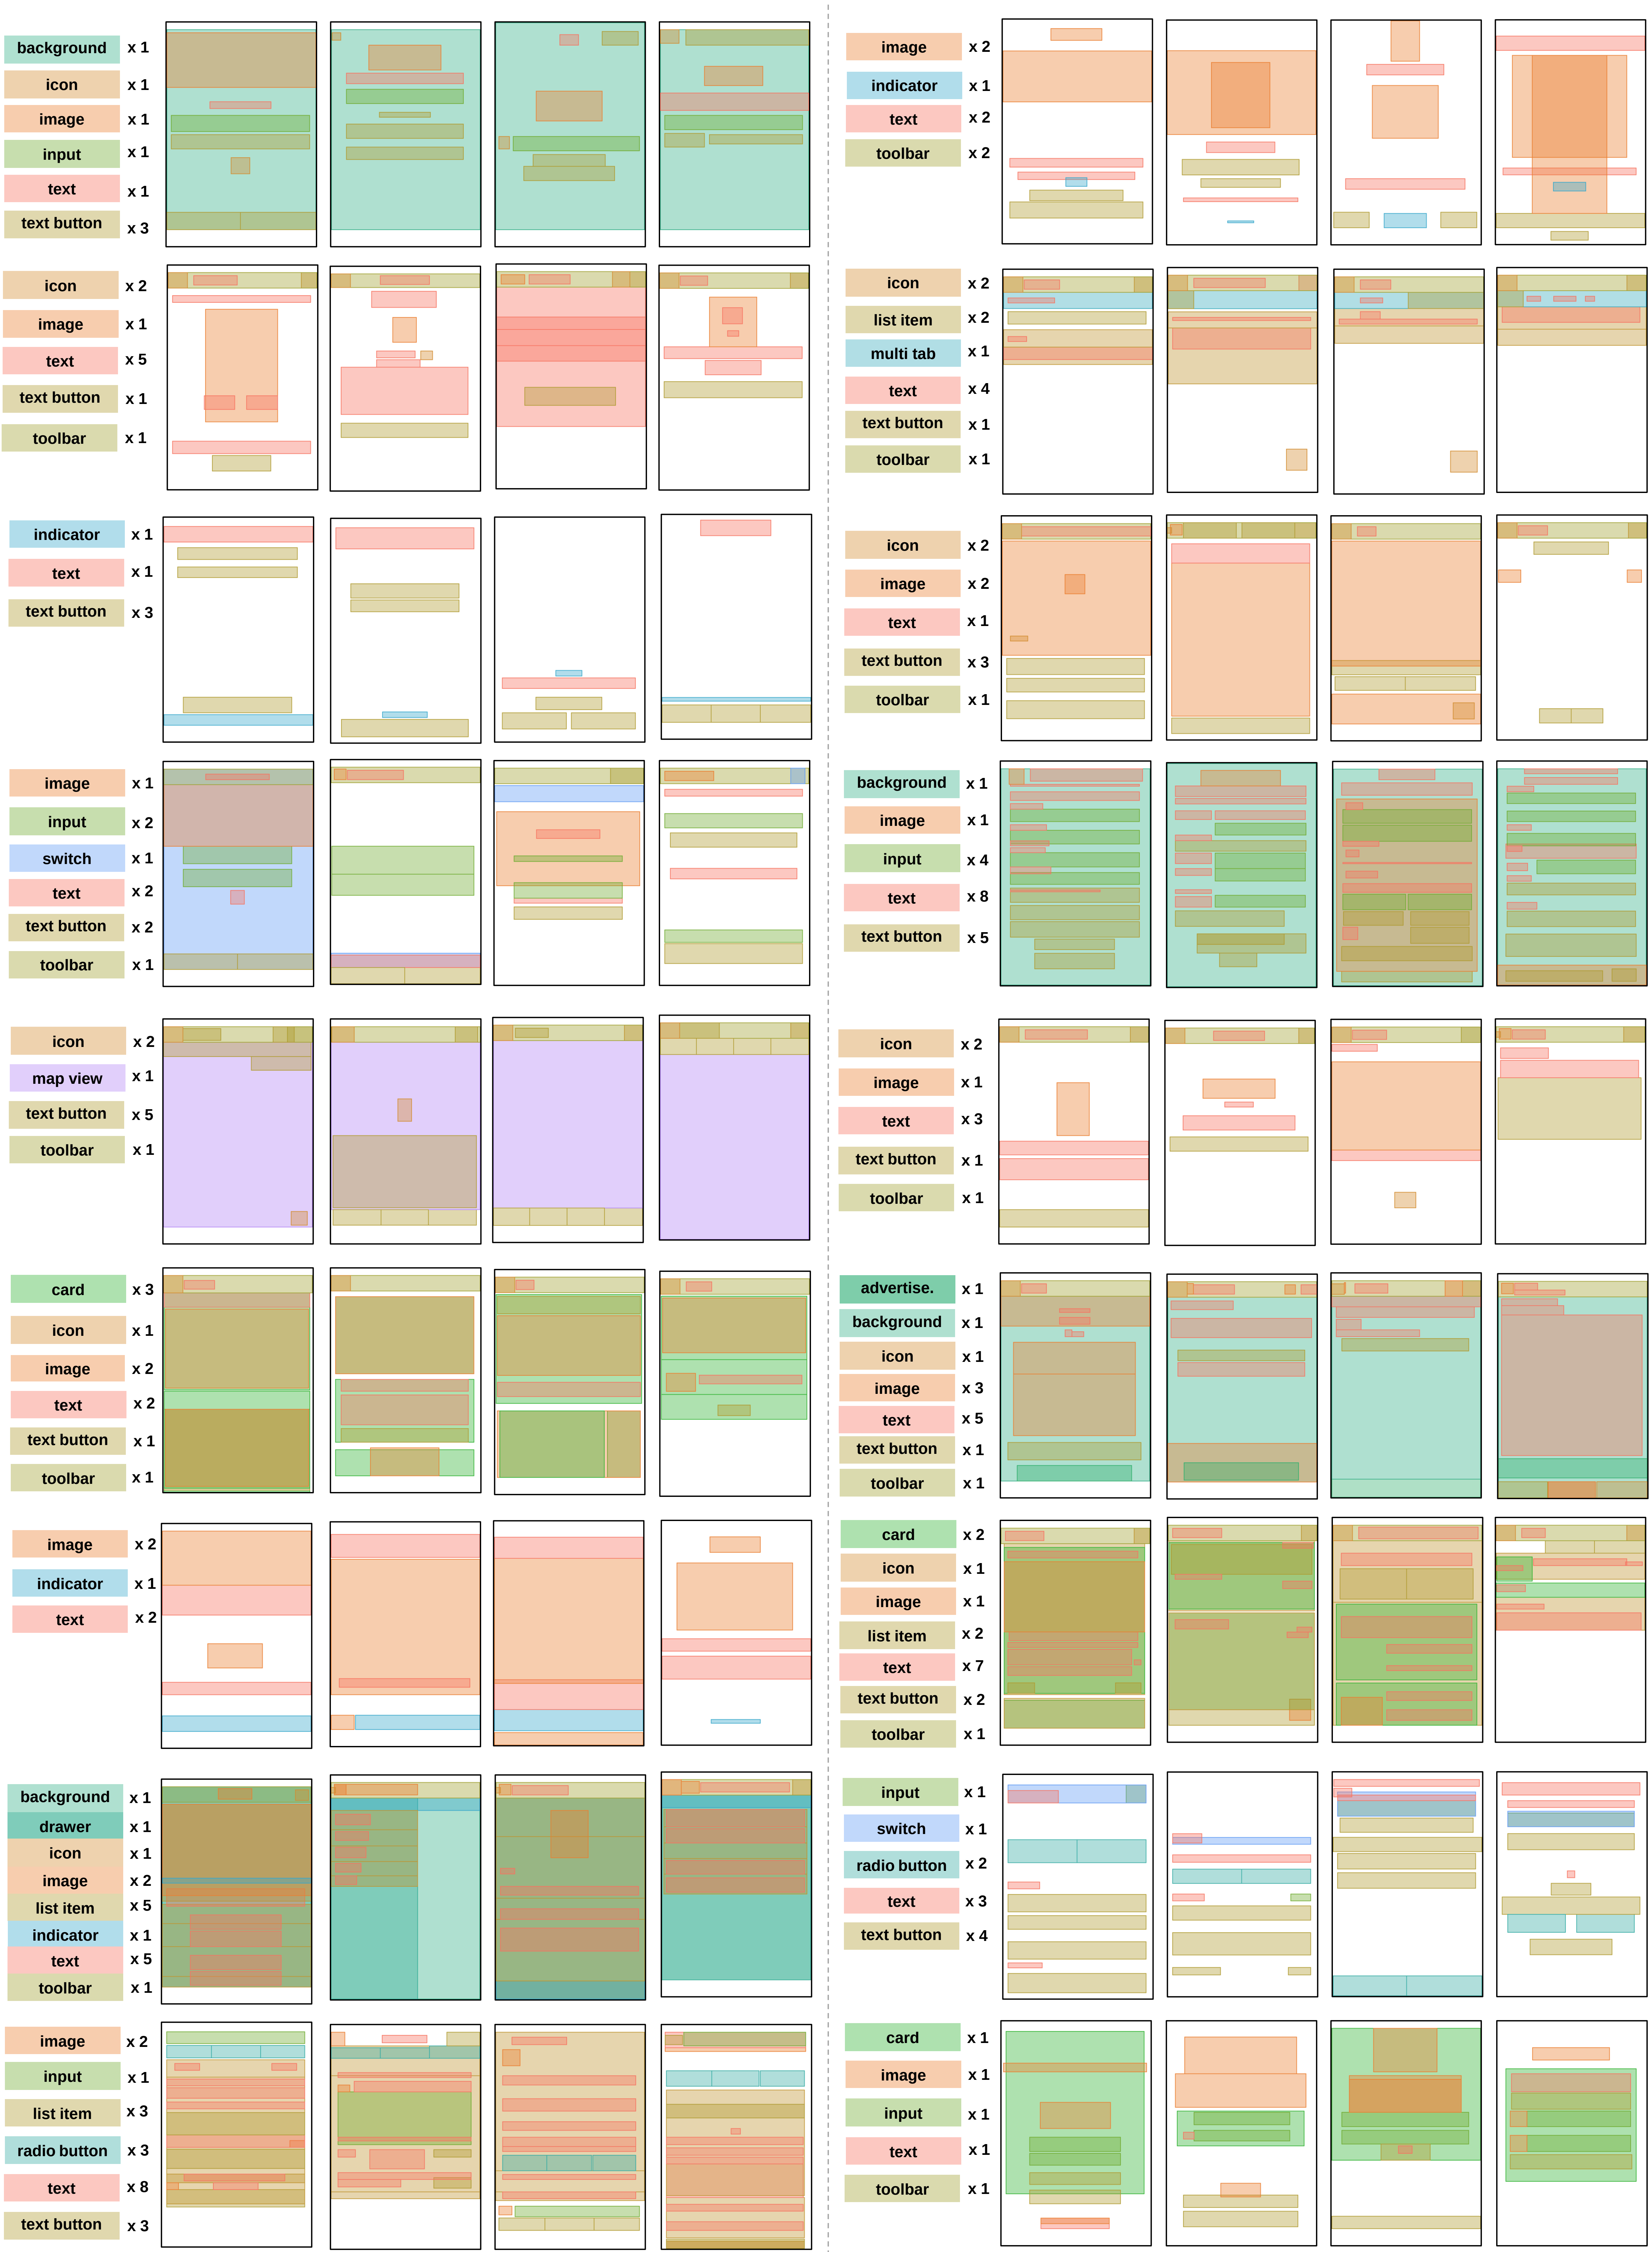
background x 1
icon x 1
image x 1
input x 1
text x 1
text button x 3
image x 2
indicator x 1
text x 2
toolbar x 2
icon x 2
image x 1
text x 5
text button x 1
toolbar x 1
icon x 2
list item x 2
multi tab x 1
text x 4
text button x 1
toolbar x 1
indicator x 1
text x 1
text button x 3
icon x 2
image x 2
text x 1
text button x 3
toolbar x 1
image x 1
input x 2
switch x 1
text x 2
text button x 2
toolbar x 1
background x 1
image x 1
input x 4
text x 8
text button x 5
icon x 2
map view x 1
text button x 5
toolbar x 1
icon x 2
image x 1
text x 3
text button x 1
toolbar x 1
card x 3
icon x 1
image x 2
text x 2
text button x 1
toolbar x 1
advertise. x 1
background x 1
icon x 1
image x 3
text x 5
text button x 1
toolbar x 1
image x 2
indicator x 1
text x 2
card x 2
icon x 1
image x 1
list item x 2
text x 7
text button x 2
toolbar x 1
background x 1
drawer x 1
icon x 1
image x 2
list item x 5
indicator x 1
text x 5
toolbar x 1
input x 1
switch x 1
radio button x 2
text x 3
text button x 4
image x 2
input x 1
list item x 3
radio button x 3
text x 8
text button x 3
card x 1
image x 1
input x 1
text x 1
toolbar x 1

| | |
|---|---|
| advertise. | x 1 |
| background | x 1 |
| card | x 1 |
| drawer | x 1 |
| icon | x 1 |
| image | x 1 |
| input | x 1 |
| indicator | x 1 |
| list item | x 1 |
| multi tab | x 1 |
| map view | x 1 |
| radio button | x 1 |
| switch | x 1 |
| text | x 1 |
| text button | x 1 |
| toolbar | x 1 |
