# Supplementary material for: LayoutDiffusion: Improving Graphic Layout Generation by Discrete Diffusion Probabilistic Models
Source: arXiv:2303.11589 source file (2023-08-15)

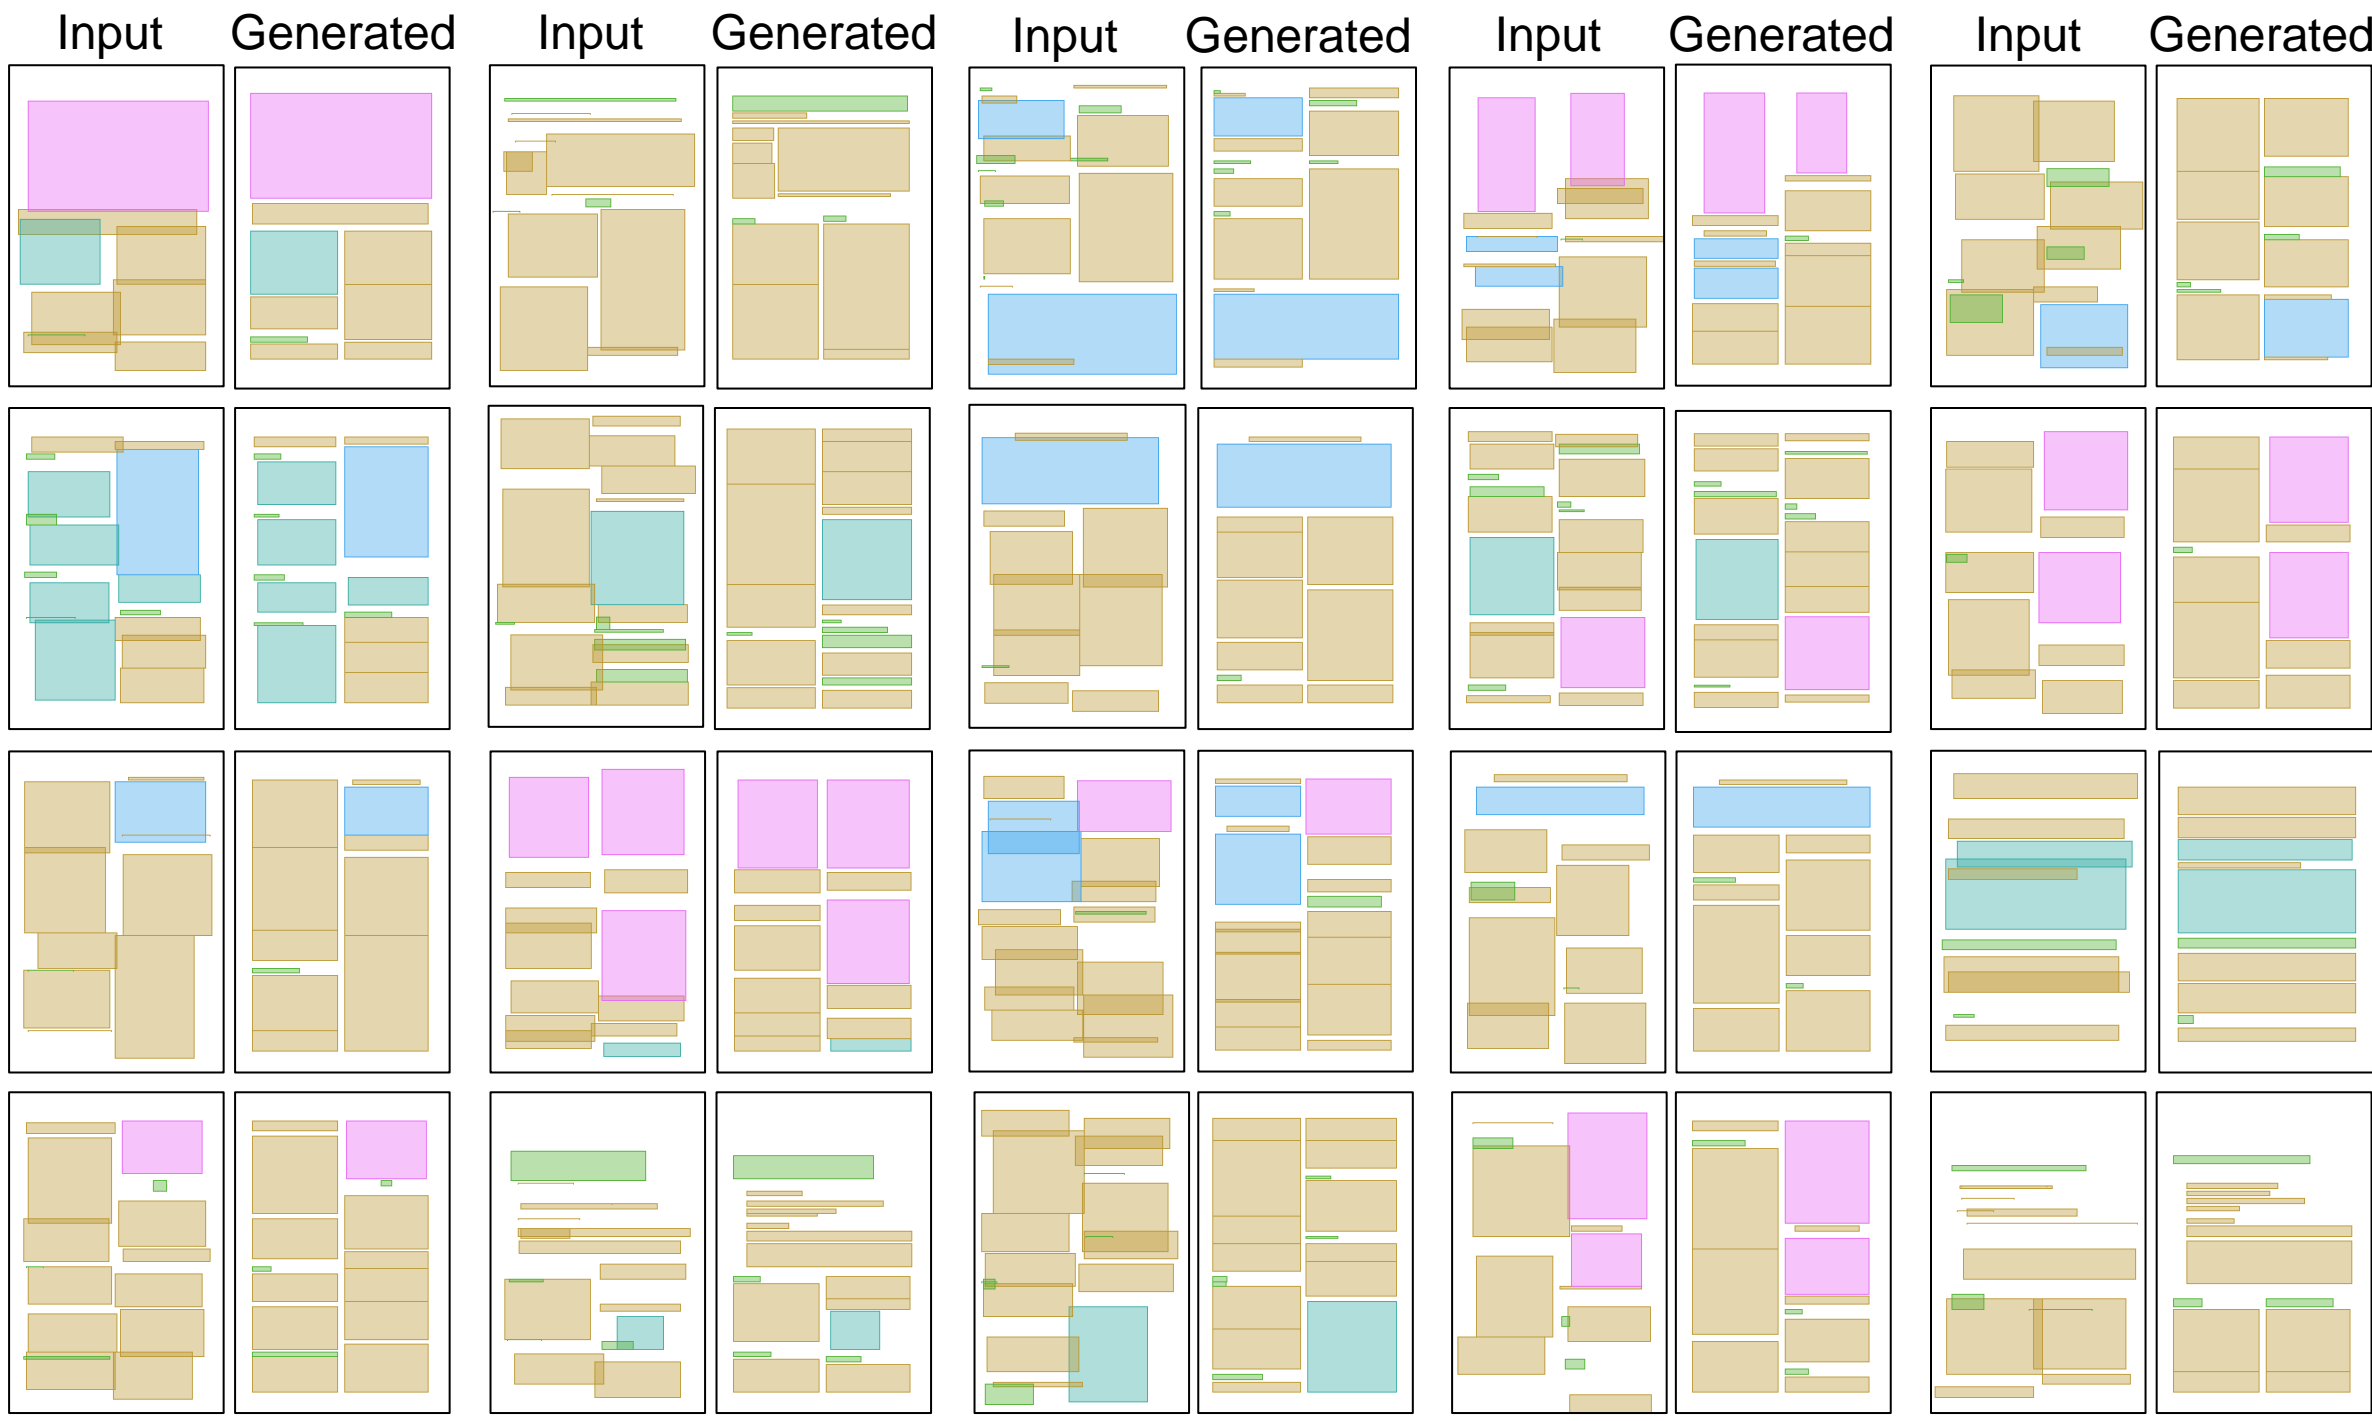

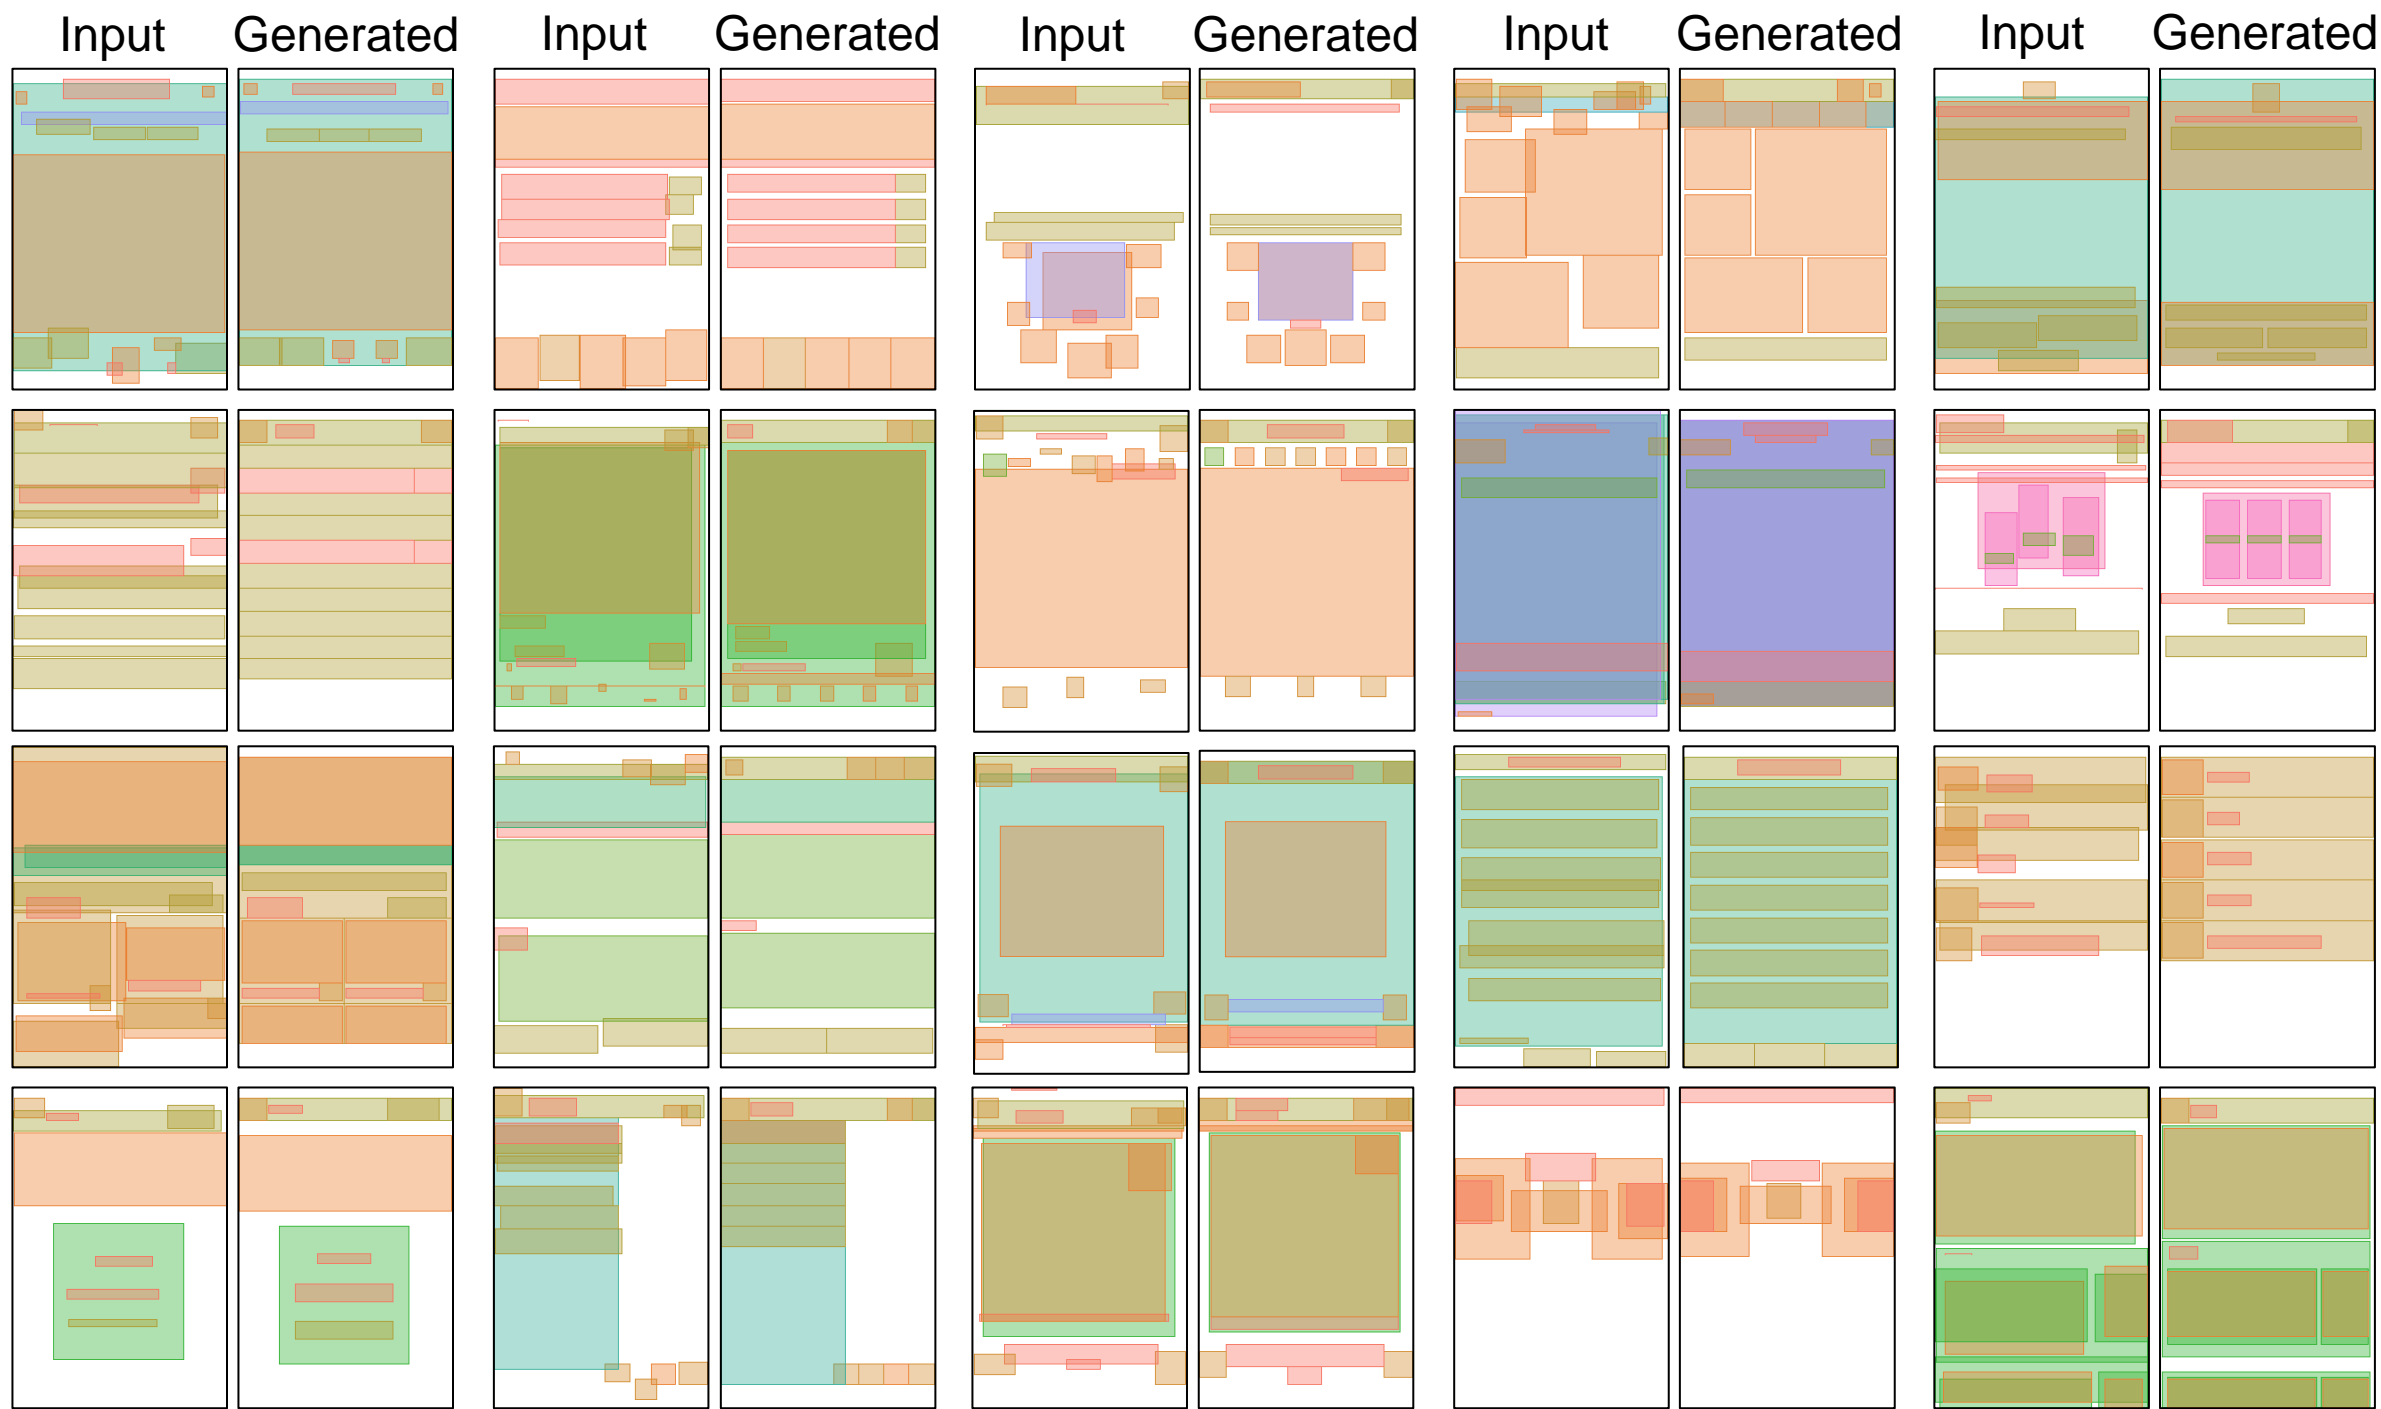

Supplement: Supplementary file 2 [file pub_refine.pdf]
