# Supplementary material for: LayoutDiffusion: Improving Graphic Layout Generation by Discrete Diffusion Probabilistic Models
Source: arXiv:2303.11589 source file (2023-08-15)
Supplement: Supplementary file 4 [file type_suppl.pdf]

Type set

LayoutFormer++

LayoutDiffusion (Ours)

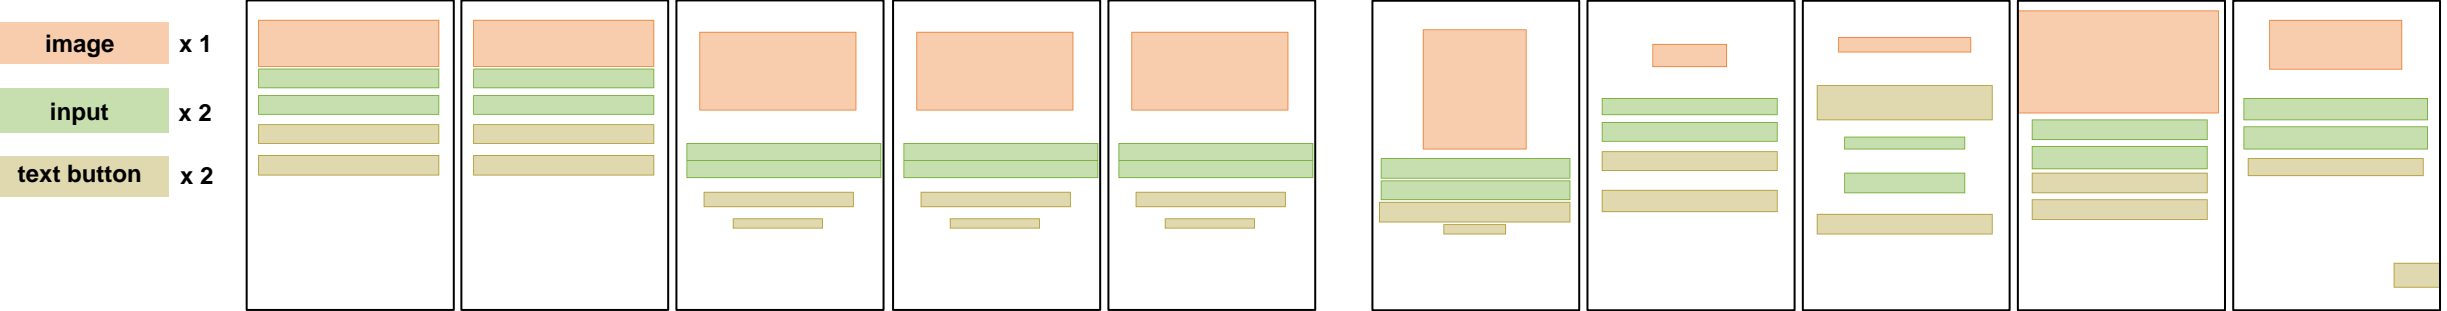

Type set

LayoutFormer++

LayoutDiffusion (Ours)

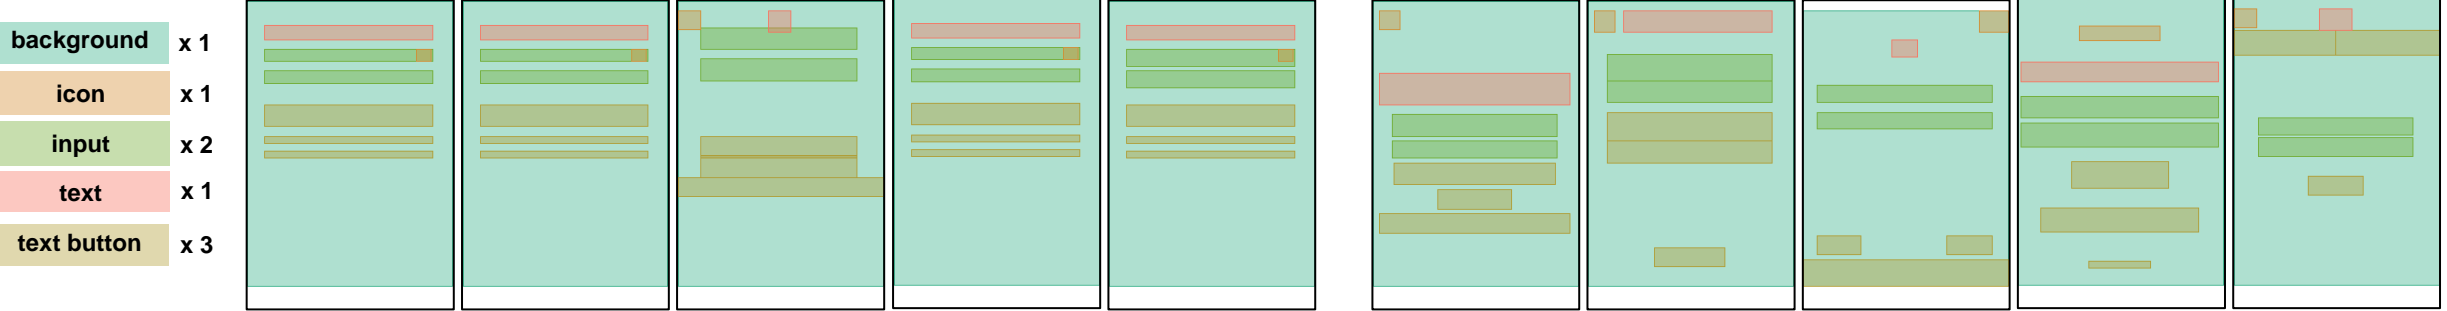

Type set

LayoutFormer++

LayoutDiffusion (Ours)

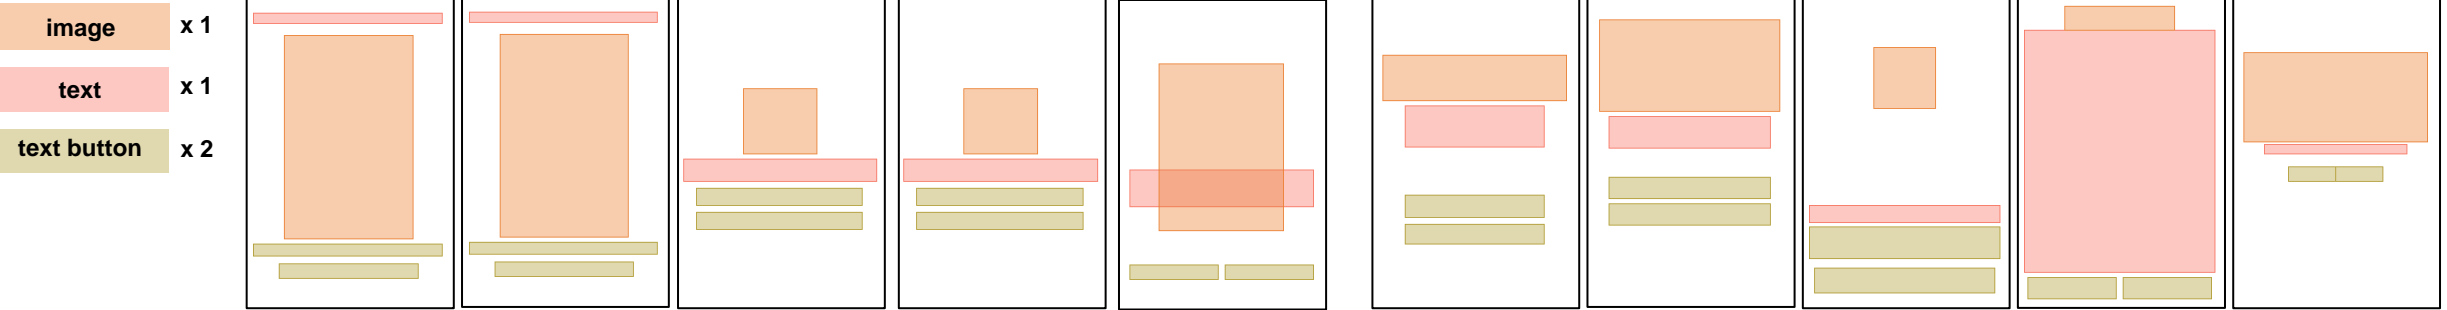

Type set

LayoutFormer++

LayoutDiffusion (Ours)

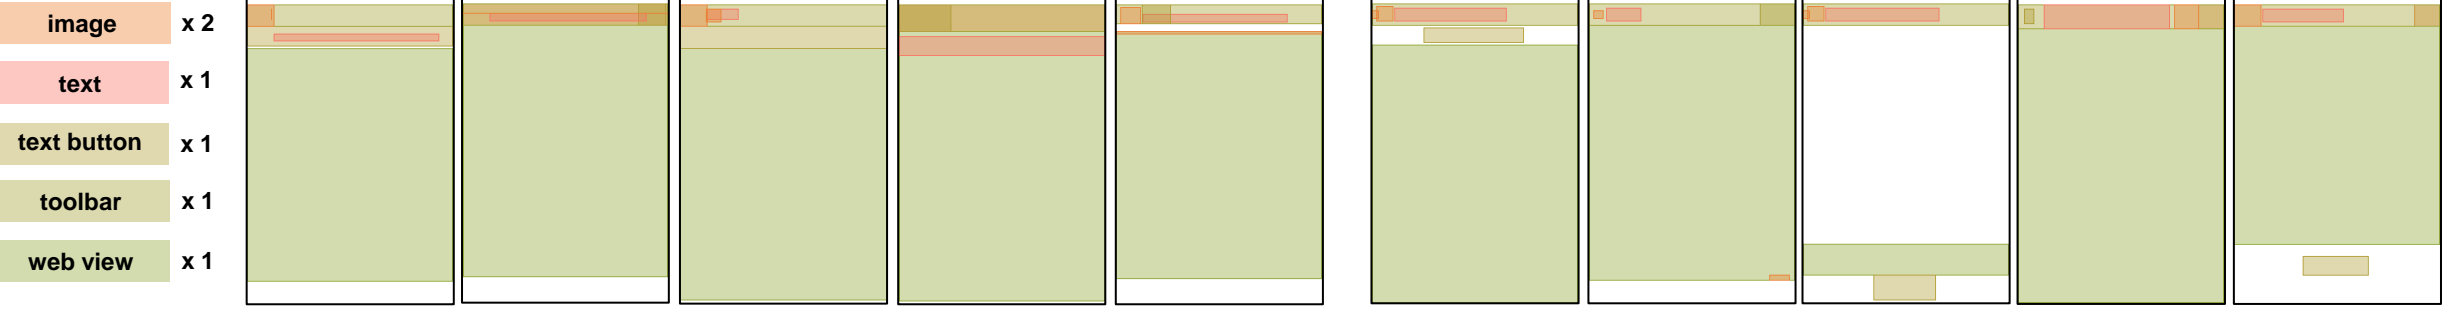

Type set

LayoutFormer++

LayoutDiffusion (Ours)

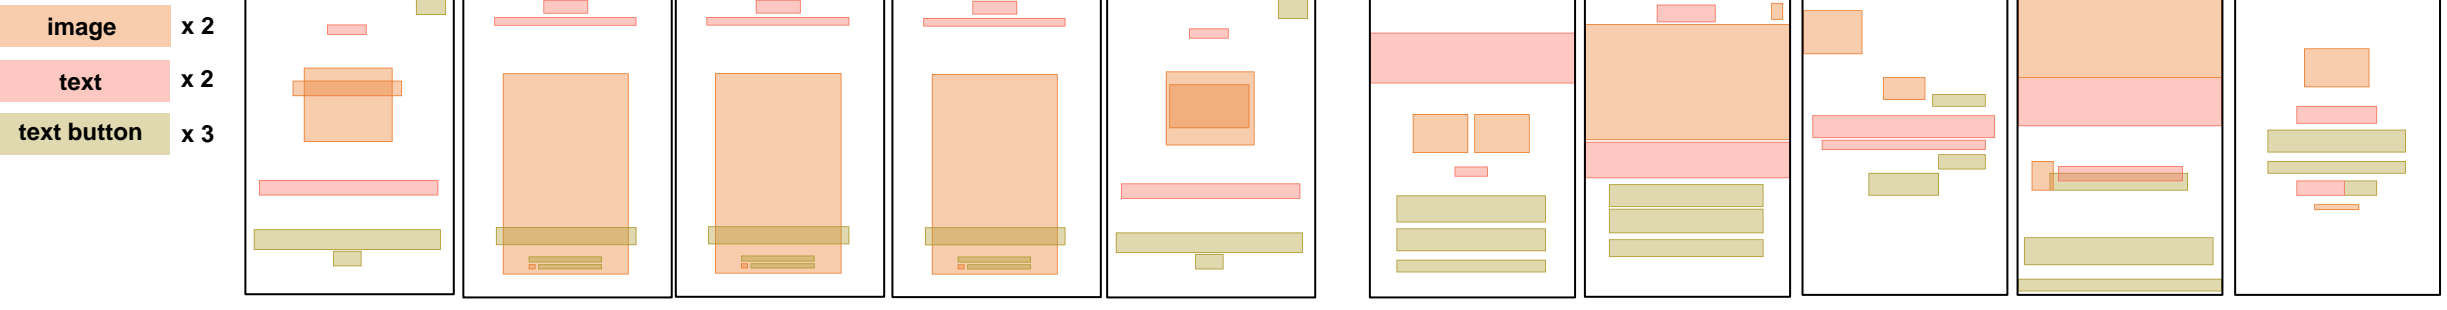

[illegible]

|              |     |
|--------------|-----|
| advertise.   | x 1 |
| background   | x 1 |
| card         | x 1 |
| drawer       | x 1 |
| icon         | x 1 |
| image        | x 1 |
| input        | x 1 |
| indicator    | x 1 |
| list item    | x 1 |
| multi tab    | x 1 |
| map view     | x 1 |
| radio button | x 1 |
| switch       | x 1 |
| text         | x 1 |
| text button  | x 1 |
| toolbar      | x 1 |
| web view     | x 1 |

[illegible][illegible]
